# Supplementary material for: Online Data Collection for Efficient Semiparametric Inference
Source: arXiv:2411.03195 source file (2024-11-05)
Supplement: Supplementary file 1 [file appendix-parametric.tex]

\begin{property}[ULLN]\label{property:mod-of-continuity}
Let $a_i(\theta) := a(X_i; \theta) \in \R$ be a continuous function
with $X_i$ sampled i.i.d. We say that $a_i(\theta)$ satisfies the ULLN property if 
(i) $\forall \theta, \, \E\left[ a_i(\theta)^2 \right] < \infty$;
(ii) $a_i(\theta)$ is dominated by a function $A(X_i)$: $\forall \theta, |a_i(\theta)| \leq A(X_i)$; and 
(iii) $\E[A(X_i)] < \infty$.
\end{property}

\begin{proposition}[MDS SLLN {\citep[Theorem~1]{csorgHo1968strong}}]\label{prop:apdx-mds-slln-general}
Let $\{ X_n, n \in \mathbb{N} \}$ be a martingale difference sequence (MDS) 
and $b_1 < b_2 < \hdots \rightarrow \infty$ be a non-decreasing sequence 
s.t. $\sum_{k=1}^{\infty} b^{-2}_k \E[X^2_k] < \infty$.
Then $b^{-1}_n \sum_{i=1}^n X_i \ConvAS 0$.
\end{proposition}

\begin{cor}[MDS SLLN]\label{cor:apdx-mds-slln}
Let $\{ X_n, n \in \mathbb{N} \}$ be a martingale difference sequence s.t. $\forall k, \,\, \E[X^2_k] < \infty$. 
Then $\frac{1}{n} \sum_{i=1}^n X_i \ConvAS 0$.
\end{cor}
\begin{proof}
Apply Prop.~\ref{prop:apdx-mds-slln-general} with $b_i= i$.
\end{proof}

\begin{lemma}[Uniform a.s. convergence]\label{lemma:apdx-uniform-convergence-dependent-data}
Let $a_i(\theta) := S_i \Tilde{a}(\theta, X_i)$ be a real-valued function where $S_i \in \{0, 1\}$ is $H_{i-1}$-measurable and $X_i$ are i.i.d. Suppose that (i) $\Theta$ is compact and (ii) $\Tilde{a}(\theta, X_i)$ satisfies Property~\ref{property:mod-of-continuity}. Then
\begin{align*}
    \sup_{\theta \in \Theta} \left| \frac{1}{T} \sum_{i=1}^T \left [ a_i(\theta) - S_i a_{*}(\theta) \right] \right| \ConvAS 0,
\end{align*}
where $a_{*}(\theta) = \E[\Tilde{a}(\theta; X_i)]$.
\end{lemma}
\begin{proof}
We follow a standard uniform law of large numbers proof (e.g. \citet[Lemma~1]{tauchen1985diagnostic}) 
and modify it to work for dependent data.
The key modification is replacing the law of large numbers (LLN) in that proof with a MDS LLN.

Let $\left( \theta_1, \theta_2, \hdots, \theta_K \right)$ be a minimal $\delta$-cover of $\Theta$ and
$N_{\delta}(\theta_k)$ denote the $\delta$-ball around $\theta_k$. 
By compactness of $\Theta$, $K$ is finite.
For $k \in [K]$ and $\theta \in N_{\delta}(\theta_k)$, we have
\begin{align*}
    & \left| \frac{1}{T} \sum_{i=1}^{T} \left[ a_i(\theta) - S_i a_{*}(\theta) \right] \right| \\
     \,\,&= \left| \frac{1}{T} \sum_{i=1}^{T} \left[ a_i(\theta) - a_i(\theta_k) + a_i(\theta_k) - S_i a_{*}(\theta_k) + S_i a_{*}(\theta_k) - S_i a_{*}(\theta) \right] \right| \\
        &\leq \frac{1}{T} \sum_{i=1}^{T} \left| a_i(\theta) - a_i(\theta_k) \right| + \left| \frac{1}{T} \sum_{i=1}^{T} \left[ a_i(\theta_k) - S_i a_{*}(\theta_k) \right] \right| + \frac{1}{T} \sum_{i=1}^{T} \left| S_i a_{*}(\theta_k) - S_i a_{*}(\theta) \right| \\
        &= \frac{1}{T} \sum_{i=1}^{T} \left| S_i \left( \Tilde{a}(\theta; X_i) - \Tilde{a}(\theta_k; X_i) \right) \right| + \left| \frac{1}{T} \sum_{i=1}^{T} \left[ a_i(\theta_k) - S_i a_{*}(\theta_k) \right] \right| + \frac{1}{T} \sum_{i=1}^{T} \left| S_i \left( a_{*}(\theta_k) - a_{*}(\theta) \right) \right| \\
        &\leq \frac{1}{T} \sum_{i=1}^{T}  \left| \Tilde{a}(\theta; X_i) - \Tilde{a}(\theta_k; X_i) \right| + \left| \frac{1}{T} \sum_{i=1}^{T} \left[ a_i(\theta_k) - S_i a_{*}(\theta_k) \right] \right| + \left| a_{*}(\theta_k) - a_{*}(\theta) \right|.
\end{align*}
We now show that each of the three terms on the RHS above is small.
In the third term, by continuity of $a_{*}(\theta)$, $\forall \epsilon > 0, \exists \delta > 0$ s.t. $\left|a_{*}(\theta_k) - a_{*}(\theta)\right| < \epsilon$.

In the second term, $\left[a_i(\theta_k) - S_i a_{*}(\theta_k; S_i)\right]$ is a MDS. 
By Property~\ref{property:mod-of-continuity}(i) and Corollary~\ref{cor:apdx-mds-slln}, we have
$ \\ \left| \frac{1}{T} \sum_{i=1}^{T} \left[ a_i(\theta_k) - S_i a_{*}(\theta_k) \right] \right| \ConvAS 0$.

Next, we examine first term on the RHS.
Let $u_i(\delta) = \sup_{\theta, \theta' \in \Theta, \left\| \theta - \theta' \right\| \leq \delta} \left| \Tilde{a}(\theta, X_i) - \Tilde{a}(\theta', X_i) \right|$.
By continuity of $\Tilde{a}(\theta, X_i)$, compactness of $\Theta$, and the Heine-Cantor theorem, $\Tilde{a}(\theta, X_i)$ is uniformly continuous in $\theta$.
This ensures that $u_i(\delta)$ is continuous in $\delta$ and thus $u_i(\delta) \downarrow 0$ as $\delta \downarrow 0$.
Since $u_i(\delta) \leq 2 A(X_i)$ (by Property~\ref{property:mod-of-continuity}(iii)), using dominated convergence, we have
$\E[u_i(\delta)] \downarrow 0$ as $\delta \downarrow 0$.
Therefore, $\forall \epsilon > 0, \exists \delta > 0$ s.t. $\E[u_i(\delta)] < \epsilon$.
Thus we can write the first term as
\begin{align*}
    \frac{1}{T} \sum_{i=1}^{T} \left| \Tilde{a}(\theta; X_i) - \Tilde{a}_i(\theta_k; X_i) \right| &\leq \frac{1}{T} \sum_{i=1}^{T} u_i(\delta) \\
        &= \frac{1}{T} \sum_{i=1}^{T} u_i(\delta) - \E[u_i(\delta)] + \E[u_i(\delta)] \\
        &\leq \frac{1}{T} \sum_{i=1}^{T} u_i(\delta) - \E[u_i(\delta)] + \epsilon \\
        &\overset{(a)}{=} o(1) + \epsilon,
\end{align*}
where (a) follows by the strong law of large numbers which applies because $E[u_i(\delta)] \leq \E[A(X_i)] < \infty$ (by Property~\ref{property:mod-of-continuity}(iii)).
\end{proof}

\begin{proposition}[Strong consistency]
Suppose that 
% (i) Assumption~\ref{assump:standard-gmm} holds, 
(ii) $\forall j \in [M], \, \Tilde{g}_{t, j}(\theta)$ satisfies Property~\ref{property:mod-of-continuity}, and
(iii) $\forall (i, j) \in [M]^2, \, \left[ \Tilde{g}_t(\theta) \Tilde{g}_t(\theta)^\top \right]_{i, j}$ satisfies Property~\ref{property:mod-of-continuity};
Then, for any policy $\pi$, $\widehat{\theta}^{(\pi)}_T \xrightarrow[T \to \infty]{a.s.} \theta^*$.
\end{proposition}
\begin{proof}
The proof goes through exactly like our previous weak consistency proof:
just replace it with the new a.s. ULLN that is proved above.
\end{proof}

\begin{lemma}[Strong consistency of $\widehat{k}_t$]\label{lemma:apdx-kappa-hat-consistency}
% Suppose that Assumption~\ref{assump:kappa-star-identify} holds.
If $\widehat{\theta}_t \ConvAS \theta^*$, then $\widehat{k}_t \ConvAS \kappa^*$ where $\widehat{k}_t = \arg\min_{\kappa \in \ChoiceSimplex} V(\widehat{\theta}_{t}, \kappa)$.
\end{lemma}
\begin{proof}
By compactness of the simplex $\Delta$ and $\widehat{\theta}_t \ConvAS \theta^*$, we have
\begin{align}
    \sup_{\kappa} \left| V(\widehat{\theta}_t, \kappa) - V(\theta^*, \kappa) \right| \ConvAS 0.
\end{align}
We also have the following three facts. For any $\epsilon > 0$,
almost surely for large enough $t$, we have
\begin{align}
    V(\widehat{\theta}_t, \widehat{k}) &< V(\widehat{\theta}_t, \kappa^*) \\
    V(\theta^*, \widehat{k}) &< V(\widehat{\theta}_t, \widehat{k}) + \epsilon \\
    V(\widehat{\theta}_t, \kappa^*) &< V(\theta^*, \kappa^*) + \epsilon.
\end{align}
Combining the above three statements, we have almost surely,
\begin{align*}
    V(\theta^*, \widehat{k}) < V(\theta^*, \kappa^*) + 2 \epsilon.
\end{align*}
By standard arguments (i.e., construct an open ball around $\kappa^*$ 
and show that $\widehat{k}$ is contained in that open set), 
we get $\widehat{k} \ConvAS \kappa^*$. 
\end{proof}

% \begin{lemma}[Strong consistency of $\widehat{k}_t$]\label{lemma:apdx-kappa-hat-consistency-estimated-variance}
% Suppose that Assumption~\ref{assump:kappa-star-identify} holds.
% If $\widehat{\theta}_t \ConvAS \theta^*$, then $\widehat{k}_t \ConvAS \kappa^*$ where $\widehat{k}_t = \arg\min_{\kappa \in \ChoiceSimplex} V(\widehat{\theta}_{t}, \kappa)$.
% \end{lemma}
% \begin{proof}
% By compactness of the simplex $\Delta$ and $\widehat{\theta}_t \ConvAS \theta^*$, we have
% \begin{align}
%     \sup_{\kappa} \left| V(\widehat{\theta}_t, \kappa) - V(\theta^*, \kappa) \right| \ConvAS 0.
% \end{align}
% We also have the following three facts. For any $\epsilon > 0$,
% almost surely for large enough $t$, we have
% \begin{align}
%     V(\widehat{\theta}_t, \widehat{k}) &< V(\widehat{\theta}_t, \kappa^*) \\
%     V(\theta^*, \widehat{k}) &< V(\widehat{\theta}_t, \widehat{k}) + \epsilon \\
%     V(\widehat{\theta}_t, \kappa^*) &< V(\theta^*, \kappa^*) + \epsilon.
% \end{align}
% Combining the above three statements, we have alomst surely,
% \begin{align*}
%     V(\theta^*, \widehat{k}) < V(\theta^*, \kappa^*) + 2 \epsilon.
% \end{align*}
% By standard arguments (i.e., construct an open ball around $\kappa^*$ 
% and show that $\widehat{k}$ is that open set), 
% we get $\widehat{k} \ConvAS \kappa^*$. 
% \end{proof}
