# Supplementary material for: Online Data Collection for Efficient Semiparametric Inference
Source: arXiv:2411.03195 source file (2024-11-05)
Supplement: Supplementary file 2 [file additional-settings.tex]

\begin{enumerate}
    \item Proxy setting with two data sources:
    (1) the first data sources gives $\{ Z, X, Y \}$, and
    (2) the second source gives $\{ W, Z \}$, where
    $W$ is a confounder and $Z$ is a proxy of the confounder
    (use the effect restoration formula).
    Not sure if the semiparametric estimator is known in this setting.
\end{enumerate}

Some possible datasets
\begin{enumerate}
    \item Neuropathic Pain Diagnosis Simulator for Causal Discovery Algorithm Evaluation
    \item Transporting Causal Effects Across Populations Using Structural Causal Modeling:An Illustration to Work-From-Home Productivity
    \item HowandWhytoUseExperimentalDatatoEvaluateMethodsforObservationalCausalInference
    \item 
\end{enumerate}
